# Supplementary material for: InTeX: Interactive Text-to-texture Synthesis via Unified Depth-aware Inpainting
Source: arXiv:2403.11878 source file (2024-03-18)
Supplement: Supplementary file 1 [file 6_appendix.tex]

\appendix

\section{More Implementation Details}

\noindent \textbf{Graphic User Interface}.
We show a screenshot of our GUI in Figure~\ref{fig:gui}. 
The left part of the GUI is a 3D viewer which allows using mouse to rotate, scale, and pan the object for free-view visualization.
The right part features the functionality of our method:
(1) In the \textit{Inpaint} panel, we allow users to set the random seed and input prompts. 
Then, users can choose to perform different actions: \textit{auto} will invoke the automatic pipeline using pre-set cameras, \textit{init} will reinitialize all the buffers, \textit{encode} will load the guidance model and encode the input prompts, \textit{inpaint} will perform inpainting on the current view, and \textit{undo} will undo the last step that changes the texture.
For post-processing, we provide the \textit{dilate} and \textit{deblur} button for padding the texture map and super-resolution. 
After finishing all the steps and satisfied with the texture, user can save the mesh to a specified path.
(2) In the \textit{Repaint} panel, users can use the mouse to draw a mask, which will erase the covered region for repainting aims.
(3) In the \textit{Render} panel, users can change the rendering mode among RGB image, depth, alpha, normal map, and view cosine map. The change of camera FOV is also supported here.

\noindent \textbf{Pre-set Cameras}.
Our 10 predefined camera poses for automatic inpainting represented with $(\text{elevation}, \text{azimuth})$ are: $(0, 0)$, $(0, 45)$, $(0, -45)$, $(0, 90)$, $(0, -90)$, $(0, 135)$, $(0, -135)$, $(0, 180)$, $(90, 0)$, $(-90, 0)$, covering 8 horizontal views, a top view, and a bottom view. We follow the same order to gradually inpaint each camera view.

\noindent \textbf{Data sources}.
All of the 3D meshes displayed in the paper are from the Objaverse~\cite{deitke2023objaverse,deitke2023objaversexl} dataset under corresponding licenses, except for the Fox and Dragon model which are from a private dataset.

\noindent \textbf{User study}.
For the user study, we render 360 degree rotating videos of 3D meshes with generated textures from different methods.
We majorly compare against open-sourced works~\cite{richardson2023texture,chen2023text2tex}.
There are in total 45 videos for 3 methods (TEXTure~\cite{richardson2023texture}, Text2tex~\cite{chen2023text2tex}, and our method) to evaluate.
Each volunteer is shown 15 samples containing the input prompt and a rendered video from a random method, and asked to rate in two aspects: 3D consistency and overall texture quality. We collect results from 30 volunteers and get 450 valid scores in total.

\section{More Results}

In Figure~\ref{fig:morecomp}, we provide more qualitative comparisons with recent methdos TEXTure~\cite{richardson2023texture} and Text2tex~\cite{chen2023text2tex}. 

\begin{figure*}[t!]
    \centering
    \includegraphics[width=\textwidth]{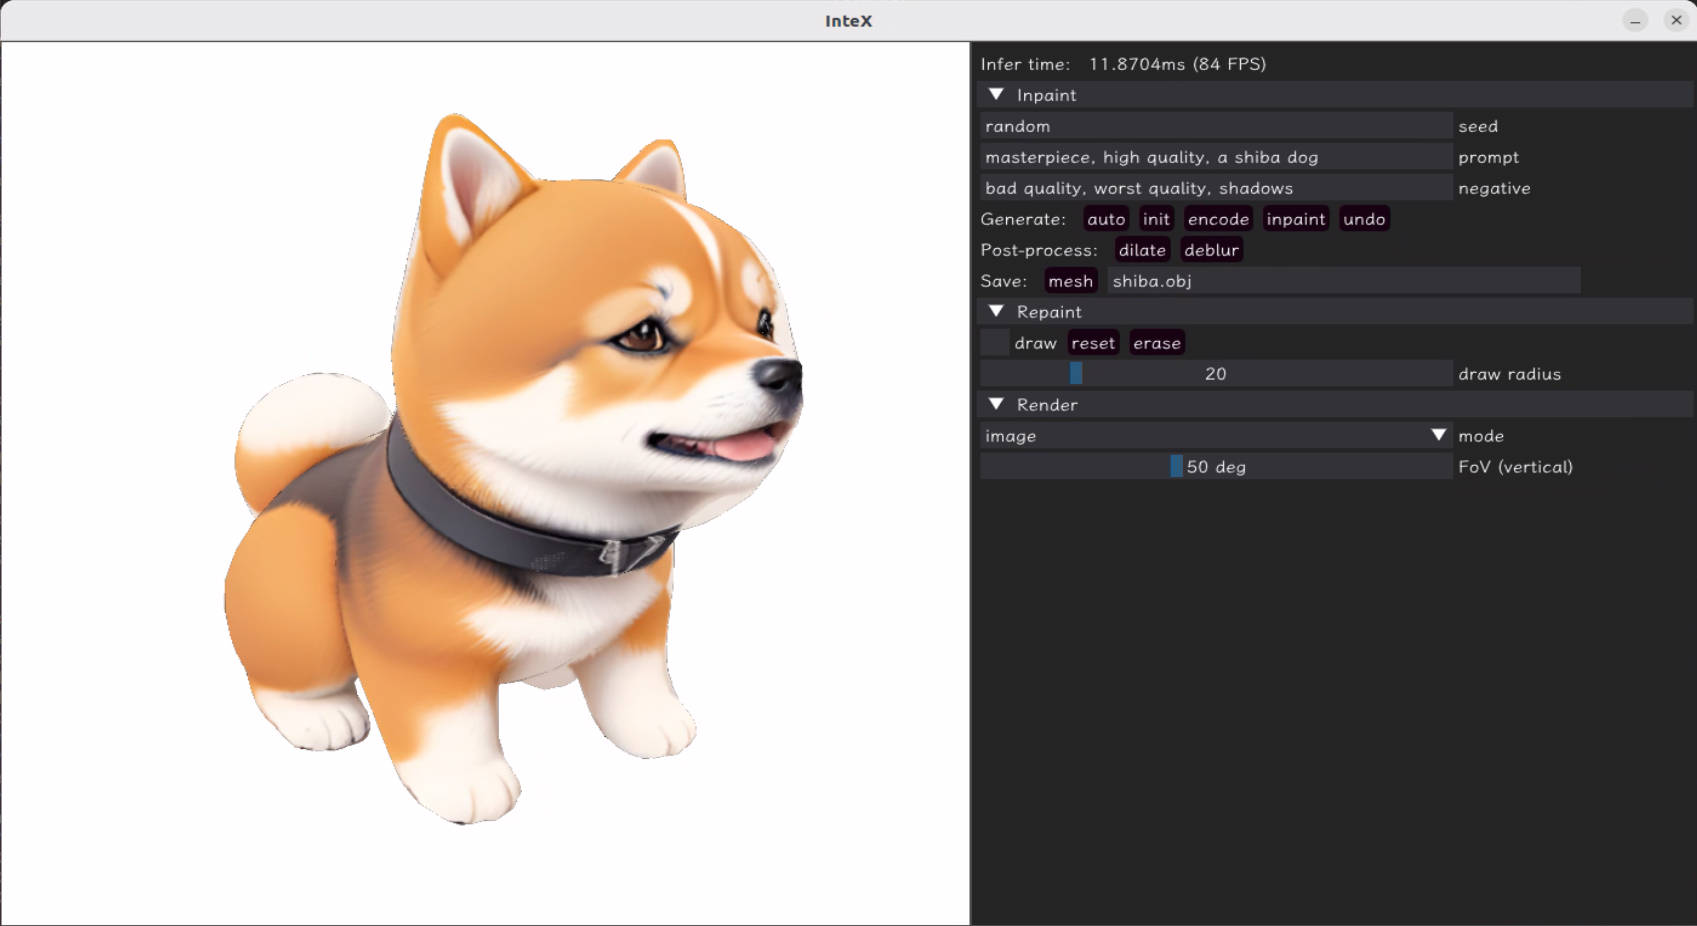}
    \caption{
    \textbf{Graphic User Interface}.
    }
    \label{fig:gui}
\end{figure*}

\begin{figure*}[t!]
    \centering
    \includegraphics[width=\textwidth]{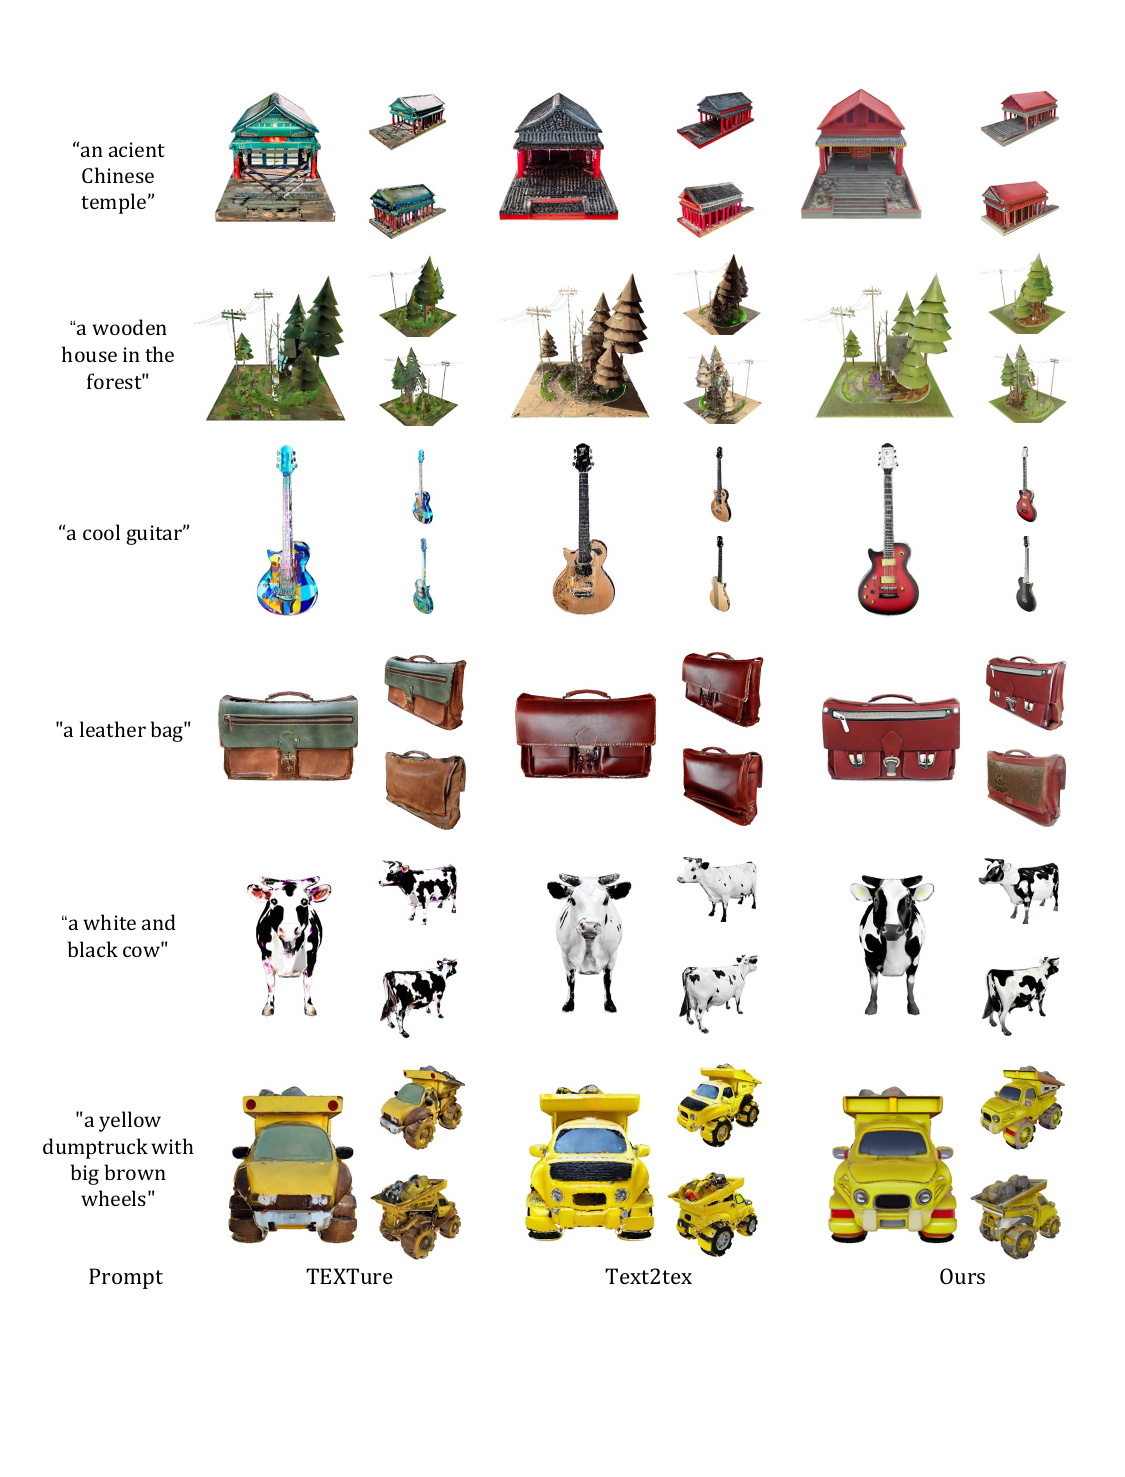}
    \caption{
    \textbf{More qualitative comparisons} of text-to-texture generation on various 3D models.
    }
    \label{fig:morecomp}
\end{figure*}
